# Supplementary material for: Competition of defect ordering and site disproportionation in strained LaCoO$_{3}$ on SrTiO$_3$(001)
Source: arXiv:2003.02317 ancillary file (2020-03-04)
Supplement: Supplementary file 1 [file Supplement.pdf]

# Competition of defect ordering and site disproportionation in strained $LaCoO_3$ on $SrTiO_3(001)$ – Supplemental Material –

Benjamin Geisler and Rossitza Pentcheva
*Fakultät für Physik, Universität Duisburg-Essen and Center for Nanointegration (CENIDE), Campus Duisburg, Lotharstr. 1, 47048 Duisburg, Germany*

## THE HIGH-SPIN STATE: HS/LS MIXTURE AND LS/LS/HS-ORDERED PLANES IN $LaCoO_3$ ON STO(001)

A frequently discussed phase of LCO bulk and films strained on STO(001) consists of a checkerboard arrangement of HS and LS sites [1–4], as displayed in Fig. 1(a). It does not show a $3 \times 1$ spin reconstruction, but it is an insulating ferromagnet. We find this phase to be considerably lower in energy than expected from bulk extrapolation [5], which is indicative of a strong stabilizing effect. This is in line with earlier PBE+$U$ results ($U_{Co} = 2.7$ eV) for bulk LCO [1]. However, the IS/IS/IS and LS/IS/IS phases of LCO films (both containing IS+CD+OO) are substantially lower in energy for all considered values of $U_{Co}$, as displayed in Figs. 1(b) and (c). This holds for both the effective-$U$ approach [6] and the rotationally invariant Liechtenstein approach [7] with $U = 4$ eV and $J = 1$ eV. The meaningful range of $U_{Co}$ is delimited (i) by the band gap of bulk LCO, which is too small for low values of $U_{Co}$, and (ii) by the destabilization of the NM LS ground state for $U_{Co} \gtrsim 4$ eV [5].

Seo *et al.* found this HS/LS mixture to be the ground state for LCO films strained on STO(001) [2], at variance with our results. This is related to their use of the LDA exchange-correlation functional ($U_{Co} = 3.8$ eV), which significantly underestimates the bulk LCO lattice constant ($a_{LCO} = 3.74$ Å instead of 3.83 Å [8]; here: 3.84 Å) due to overbinding. Consequently, the LCO films are under far higher tensile epitaxial strain in their simulations (3.5 %) compared to experiments or our PBE simulations (2 %) if matched to the STO lattice constant of 3.905 Å.

Kwon *et al.* suggested a LS/LS/HS $3 \times 1$ spin reconstruction to arise in stoichiometric LCO films [9]. In our large supercells and with explicit treatment of octahedral rotations (which are known to strongly impact the magnetic properties in LCO [5]), this phase could only be obtained under application of constraints to the total magnetization. Once these constraints were lifted, the HS Co ions relaxed to the IS state. Thus, the LS/LS/HS phase is not even metastable. We attribute the different observations to the small supercells and the neglect of octahedral rotations in previous work.

Figure 1(c) shows that around $U_{Co} = 3$ eV there is a close competition between the IS/IS/IS and the LS/IS/IS phase, i.e., the energy difference between these phases amounts to only a few meV/Co. This allows external influences (e.g., dilute impurities such as oxygen vacancies, TEM sample preparation conditions, proximity effects of differently magnetized domains, or the polarity of the LCO/STO(001) interface) to impact which phase stabilizes. This might constitute a part of the puzzle why the $3 \times 1$ reconstruction of LCO films strained on STO(001) is sometimes *not* observed [10, 11].

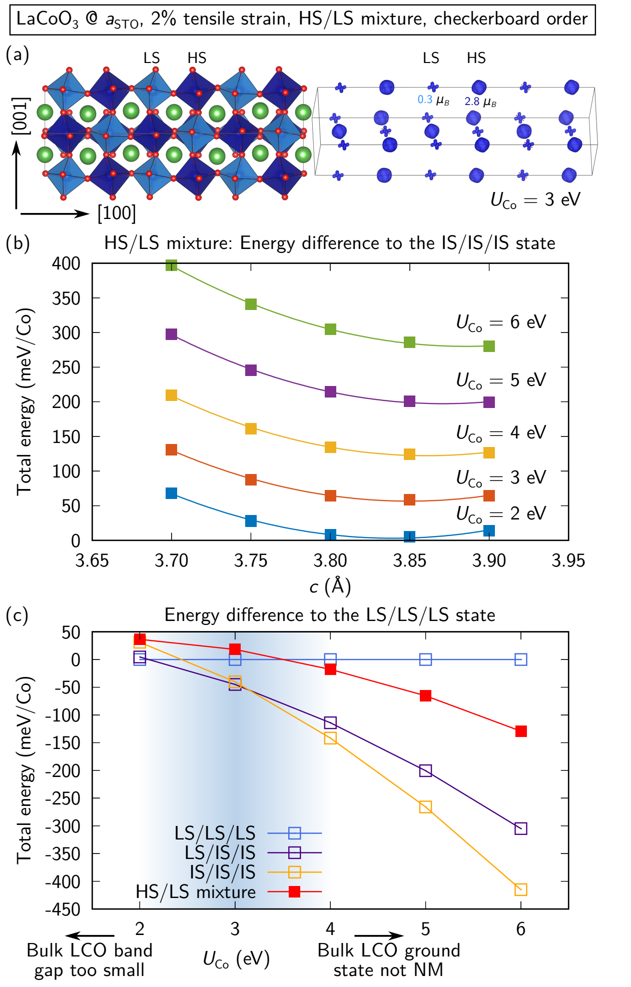


Figure 1. (a) Optimized structure and spin density of LCO films strained on STO(001) in the mixed HS/LS phase. (b) Total energy difference as function of the $c$ lattice parameter of the mixed HS/LS phase to the site-disproportionated and orbital-ordered IS/IS/IS phase for different values of $U_{Co}$. (c) Relative stability of different magnetic phases of LCO films strained on STO(001) as function of $U_{Co}$. The shaded area indicates the meaningful range of $U_{Co}$.

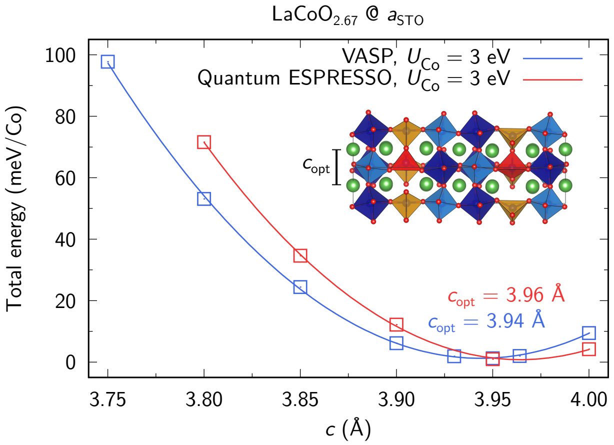


Figure 2. Optimization of the vertical $c$ lattice parameter for $LaCoO_{2.67}$ films strained on STO(001), comparing Quantum ESPRESSO and VASP. The vertical expansion due to oxygen vacancies reported in the present paper is consistently provided within an error bar of $\pm 0.01$ Å by both approaches, despite their technical differences.

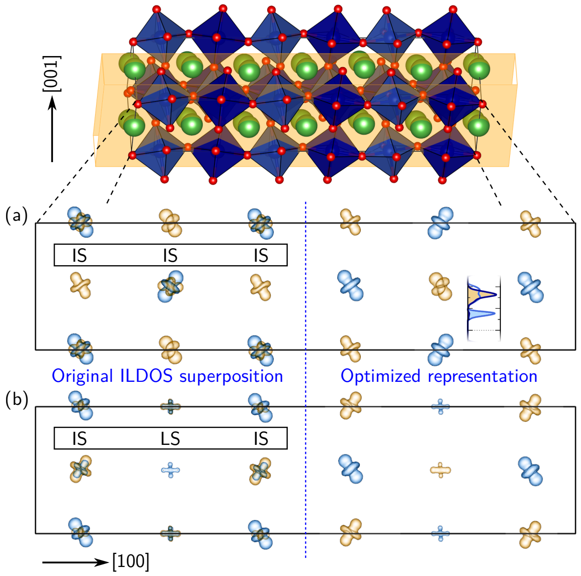


Figure 3. Reproduction of Fig. 6 from the main text, comparing original results and the optimized graphical representation.

## $LaCoO_{2.67}$ ON STO(001): COMPARISON OF QUANTUM ESPRESSO AND VASP

In the present paper, we report an increasing vertical expansion of LCO films strained on STO(001) with increasing oxygen vacancy concentration, which goes hand in hand with a partial Co reduction. This can be understood from the ionic radius of HS Co, which is considerably larger than that of LS Co [2]. Hence, HS Co sites are enclosed in larger $CoO_6$ octahedra than LS Co sites, which implies a vertical expansion if the basal lattice parameters are fixed by the STO substrate. Additional calculations employing the Vienna Ab initio simulation package [12–14] (VASP) clearly confirmed this finding (Fig. 2), despite the technical differences (ultrasoft pseudopotentials vs. projector augmented wave method, different projectors to construct occupation matrix in the DFT+$U$ formalism).

## $LaCoO_{2.83}$ ON STO(001)

Recently, Fumega and Pardo reported a $LaCoO_{2.83}$ phase [15], which shows good structural agreement with the experimentally measured $3 \times 1$ reconstruction [16]. It constitutes an intermediate concentration of oxygen vacancies between the perovskite $LaCoO_3$ and $LaCoO_{2.67}$ phases discussed in the present paper. In this phase, HS $Co^{2+}$ ions arise solely in the oxygen-vacancy planes, whereas the remaining sites are $Co^{3+}$; this is distinct from the $LaCoO_{2.67}$ model [16]. We reproduced their results within our methodology, finding an optimized cell height of $c_{opt} = 3.82$ Å. However, our thermodynamic analysis (Fig. 9 in the main text) shows that this structure is substantially less stable than $LaCoO_3$ or $LaCoO_{2.67}$, irrespective of the growth conditions.


[1] K. Knížek, Z. c. v. Jirák, J. c. v. Hejtmánek, P. Novák, and W. Ku, Phys. Rev. B **79**, 014430 (2009).

[2] H. Seo, A. Posadas, and A. A. Demkov, Phys. Rev. B **86**, 014430 (2012).

[3] H. Hsu, P. Blaha, and R. M. Wentzcovitch, Phys. Rev. B **85**, 140404 (2012).

[4] G. E. Sterbinsky, R. Nanguneri, J. X. Ma, J. Shi, E. Karapetrova, J. C. Woicik, H. Park, J.-W. Kim, and P. J. Ryan, Phys. Rev. Lett. **120**, 197201 (2018).

[5] J. M. Rondinelli and N. A. Spaldin, Phys. Rev. B **79**, 054409 (2009).

[6] M. Cococcioni and S. de Gironcoli, Phys. Rev. B **71**, 035105 (2005).

[7] A. I. Liechtenstein, V. I. Anisimov, and J. Zaanen, Phys. Rev. B **52**, R5467 (1995).

[8] P. G. Radaelli and S.-W. Cheong, Phys. Rev. B **66**, 094408 (2002).

[9] J.-H. Kwon, W. S. Choi, Y.-K. Kwon, R. Jung, J.-M. Zuo, H. N. Lee, and M. Kim, Chem. Mat. **26**, 2496 (2014).

[10] L. Qiao, J. H. Jang, D. J. Singh, Z. Gai, H. Xiao, A. Mehta, R. K. Vasudevan, A. Tselev, Z. Feng, H. Zhou, S. Li, W. Prellier, X. Zu, Z. Liu, A. Borisevich, A. P. Baddorf, and M. D. Biegalski, Nano Lett. **15**, 4677 (2015).

[11] Q. Feng, D. Meng, H. Zhou, G. Liang, Z. Cui, H. Huang, J. Wang, J. Guo, C. Ma, X. Zhai, Q. Lu, and Y. Lu, Phys. Rev. Materials **3**, 074406 (2019).

[12] P. E. Blöchl, Phys. Rev. B **50**, 17953 (1994).

[13] G. Kresse and J. Furthmüller, Phys. Rev. B **54**, 11169 (1996).

[14] G. Kresse and D. Joubert, Phys. Rev. B **59**, 1758 (1999).

[15] A. O. Fumega and V. Pardo, Phys. Rev. Materials **1**, 054403 (2017).

[16] N. Biškup, J. Salafranca, V. Mehta, M. P. Oxley, Y. Suzuki, S. J. Pennycook, S. T. Pantelides, and M. Varela, Phys. Rev. Lett. **112**, 087202 (2014).
